# Supplementary material for: Sub-Standards and Mal-Practices: Misinformation's Role in Insular, Polarized, and Toxic Interactions on Reddit
Source: arXiv:2301.11486 source file (2024-10-30)
Supplement: Supplementary file 1 [file appendix.tex]

\newpage
\section{Alternative MediaFact Distributions\label{sec:mediafact-toxicity-polarizations}}
Here we present the toxicity and political ideological distribution among commenters on submissions that linked to our second set of 835~misinformation domains and 1,720~authentic news websites. 

\begin{figure*}
\begin{subfigure}{.4\textwidth}
  \centering
  \includegraphics[width=1\linewidth]{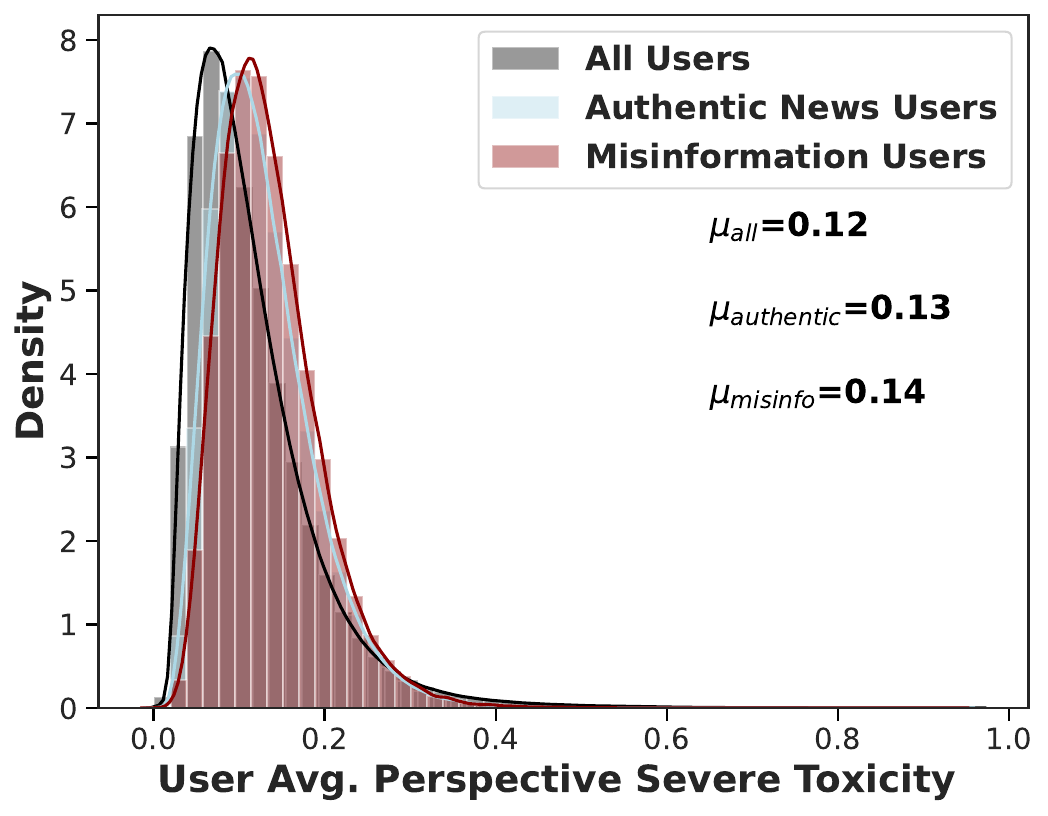}
    \caption{User Toxicity}
  \label{fig:pagerank-sub2}
\end{subfigure}
\begin{subfigure}{.42\textwidth}
  \centering
  \includegraphics[width=1\linewidth]{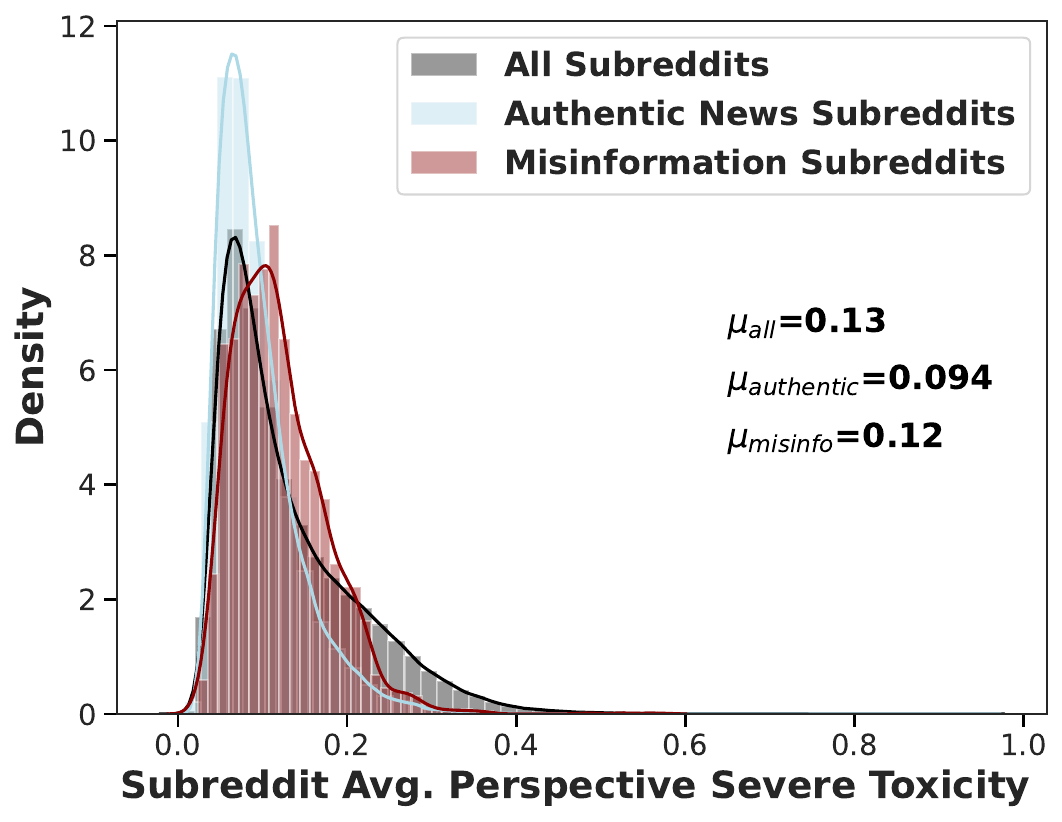}
      \caption{Subreddit Toxicity}
  \label{fig:pagerank-sub2}
\end{subfigure}
\caption{{Toxicity levels for users who comment under authentic News and misinformation URL Reddit submissions}---Users who interact with misinformation submissions are slightly more toxic/uncivil than users that interact with authentic news. Both groups are slightly more toxic/uncivil than Reddit users generally. Similarly, subreddits with misinformation submissions are overall more toxic/uncivil compared with authentic news subreddits and subreddits more generally. }
\label{fig:users-misinformation-authentic-toxicity2}
\end{figure*}
\subsection{Differences in Toxicity/Incivility between Misinformation and Authentic News Submissions\label{sec:appendix-toxicity}}

Across our second set of 9,558~misinformation and 560,673~authentic news submissions, we see a similar pattern of higher toxicity in the misinformation submission comments. 15.3\% of the misinformation submissions had toxic comments with 1.25\% of the comments being toxic. In contrast, 11.74\% of the mainstream submissions had toxic comments with 0.64\% of the comments being toxic. We thus see in this replicated experiment that Reddit misinformation conversations indeed have a higher incidence and occurrence of toxicity and incivility.

\begin{figure*}
 
 \begin{subfigure}{.4\textwidth}
  \centering
\includegraphics[width=1\linewidth]{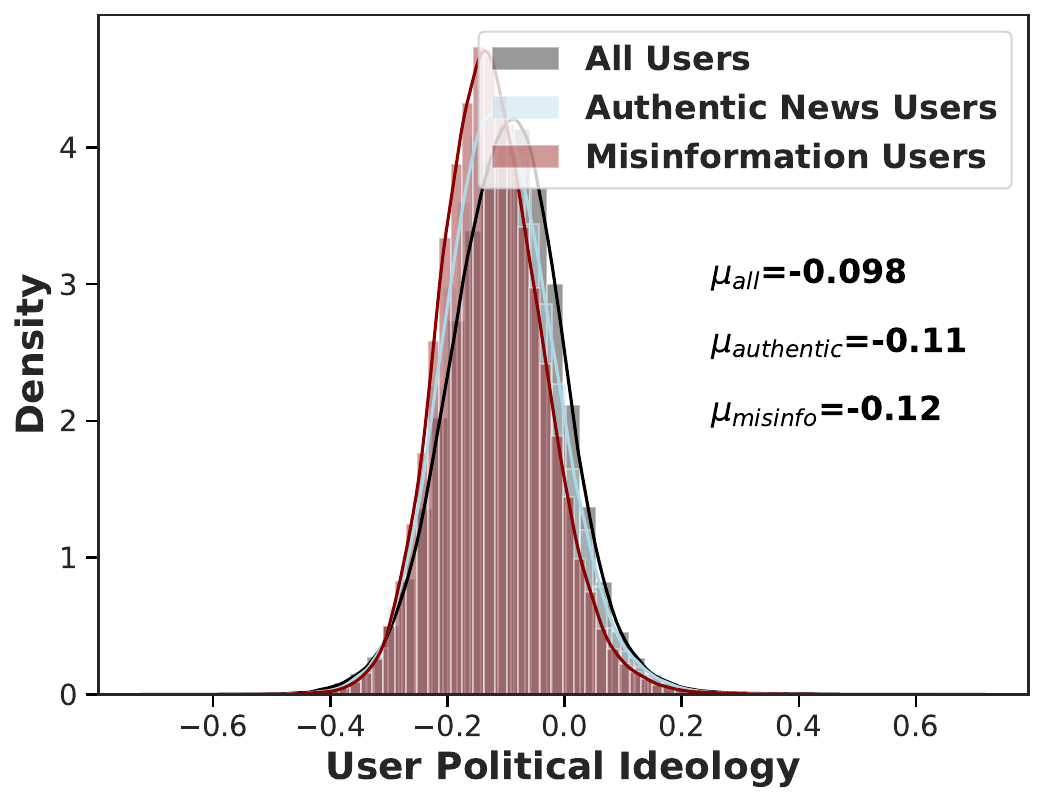}
    \caption{User Political Ideology}
  \label{fig:pagerank-sub2}
\end{subfigure}
\begin{subfigure}{.4\textwidth}
  \centering
\includegraphics[width=1\linewidth]{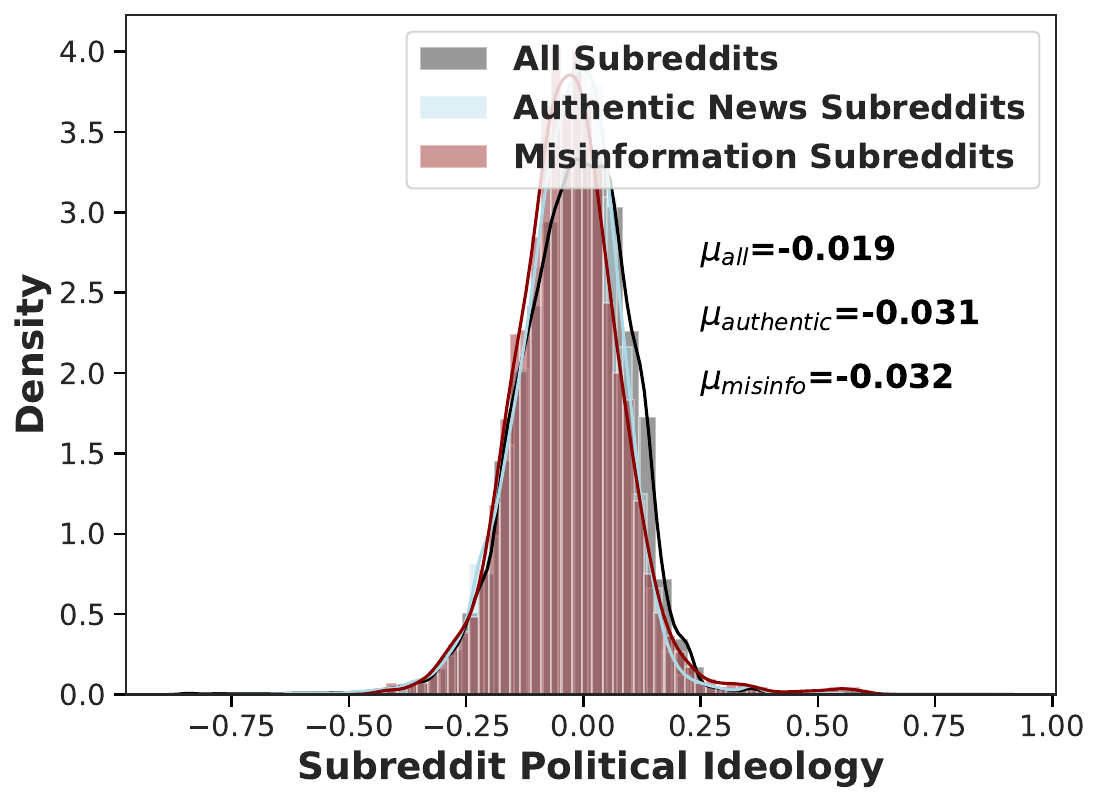}
    \caption{Subreddit Political Ideology}
  \label{fig:pagerank-sub2}
\end{subfigure}

\caption{{Political Ideology of subreddits with authentic news and misinformation Reddit submissions}--- There are no significant differences in political ideology between users who comment on misinformation and those that comment on authentic news. Similarly, there are no significant differences in the political orientation of subreddits where misinformation and authentic news appear.}
\label{fig:subreddit-political-authentic2}
\end{figure*}
 
 \begin{figure}
\centering
\begin{subfigure}{.4\textwidth}
  \centering
\includegraphics[width=1\linewidth]{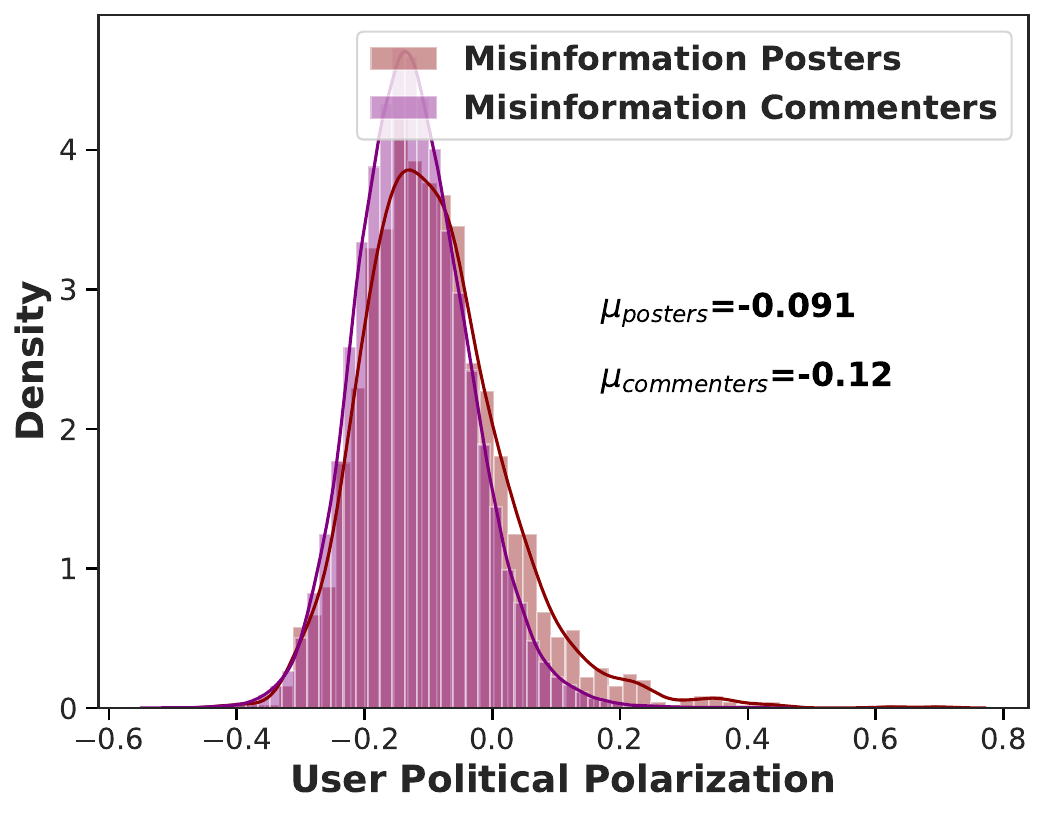}
    \caption{Misinformation}
\end{subfigure}
\begin{subfigure}{.4\textwidth}
  \centering
\includegraphics[width=1\linewidth]{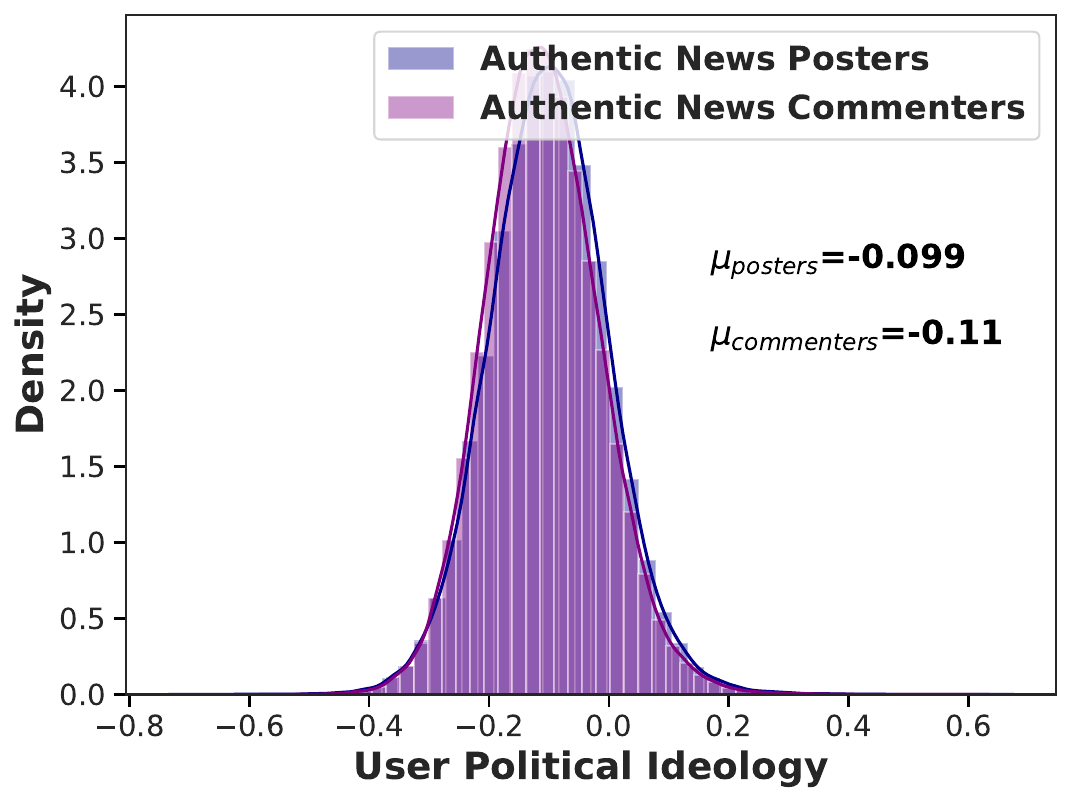}
    \caption{Authentic News}
\end{subfigure}
\caption{{Political Ideology of posters and commenters of misinformation}--- There is a noticeable rightward tilt in users who post misinformation compared to those who comment on misinformation. Unlike misinformation posts, the posters and the commenters on authentic news share similar distributions of political ideology.\label{figure:misinformation-posters-commenters2}}

\end{figure}
 
Similarly, on average 1.48\% of all comments posted by the second group of misinformation commenters are toxic compared to 1.32\% for the authentic news commenters (Figure~\ref{fig:users-misinformation-authentic-toxicity2}). Looking at the subreddits where these misinformation and authentic news submissions are posted, we again see a similar trend  (1.1\% toxic comments vs. 0.7\% toxic comments). 

\subsection{Differences in Political Ideology between Misinformation and Authentic News Submissions}\label{sec:appendix-polarization}

Again examining the political ideology of users commenting under misinformation Reddit submissions, we surprisingly do not see dramatic differences between them and users that comment on authentic news submissions. Similarly again looking in Figure~\ref{fig:subreddit-political-authentic2} at the political orientation of the subreddits where our misinformation submissions appeared, we again see that there is not much difference in their respective political ideology distributions.

We note that despite misinformation appearing in subreddits across the political spectrum, the users who post misinformation have a rightward tilt compared to the users who comment on misinformation. As seen in Figure~\ref{figure:misinformation-posters-commenters2}, misinformation submitters are on the whole more conservative than their corresponding more liberal commenters. This again is largely in contrast to authentic news commenters and posters.
